# Supplementary material for: BiSHop: Bi-Directional Cellular Learning for Tabular Data with Generalized Sparse Modern Hopfield Model
Source: arXiv:2404.03830 source file (2024-07-12)
Supplement: Supplementary file 1 [file additional_exp_table.tex]

\begin{table*}[ht]
\centering
\caption{Additional Datasets: Categorical Classification}
\resizebox{\textwidth}{!}{%
\begin{tabular}{@{}lcccccccc@{}}
\toprule
   Dataset ID &             BiSHop &     FT Transformer & GradientBoostingTree &       MLP & RandomForest &    Resnet &     SAINT &            XGBoost \\
\midrule
       361110 &          82.85 (6) &           83.2 (5) &            88.15 (2) & 82.42 (8) &    87.69 (3) & 82.65 (7) & 83.23 (4) & \textbf{88.61 (1)} \\
       361111 &          61.07 (4) &           60.0 (7) &            64.67 (3) & 60.54 (6) &    66.21 (2) & 59.97 (8) & 60.56 (5) & \textbf{66.85 (1)} \\
       361113 &          82.96 (8) &          85.93 (2) &            85.43 (4) & 83.32 (7) &    85.86 (3) & 83.96 (6) & 85.33 (5) & \textbf{86.58 (1)} \\
       361282 & \textbf{66.08 (1)} &          65.63 (4) &            65.76 (2) & 65.32 (7) &    65.53 (5) & 65.23 (8) & 65.52 (6) &           65.7 (3) \\
       361283 & \textbf{72.69 (1)} &           71.9 (5) &            72.09 (3) & 71.41 (7) &    72.13 (2) &  71.4 (8) &  71.9 (5) &          72.08 (4) \\
       361285 &          76.54 (4) & \textbf{77.09 (1)} &            76.31 (5) & 75.59 (8) &    76.13 (6) & 76.09 (7) & 76.69 (3) &          76.89 (2) \\
       361286 &  \textbf{69.8 (1)} &          68.97 (4) &            68.62 (6) & 69.06 (2) &    68.49 (7) &  69.0 (3) & 68.87 (5) &           68.2 (8) \\
\midrule
Average Score &              73.14 &              73.25 &                74.43 &     72.52 &        74.58 &     72.61 &     73.16 &              74.99 \\
 Average Rank &               3.57 &                4.0 &                 3.57 &      6.43 &          4.0 &      6.71 &      4.71 &               2.86 \\
\bottomrule
\end{tabular}
}
\end{table*}

\begin{table*}[ht]
\centering
\caption{Additional Datasets: Numerical Classification}
\resizebox{\textwidth}{!}{%
\begin{tabular}{@{}lcccccccc@{}}
\toprule
   Dataset ID &             BiSHop & FT Transformer & GradientBoostingTree &       MLP &       RandomForest &    Resnet &              SAINT &            XGBoost \\
\midrule
       361055 & \textbf{78.29 (1)} &      77.73 (2) &            77.52 (4) & 77.41 (5) &          76.35 (7) & 77.53 (3) &          77.41 (5) &          75.91 (8) \\
       361060 &           80.9 (7) &      81.95 (5) &            86.58 (2) & 80.89 (8) &          86.27 (3) & 81.16 (6) &          81.97 (4) &  \textbf{86.9 (1)} \\
       361061 &          76.91 (8) &      80.58 (5) &            81.61 (3) & 78.06 (7) &  \textbf{82.8 (1)} &  79.7 (6) &           80.6 (4) &          81.79 (2) \\
       361062 & \textbf{98.82 (1)} &       98.5 (2) &            98.16 (6) &  94.7 (8) &          98.24 (4) & 95.22 (7) &          98.21 (5) &          98.35 (3) \\
       361063 &          88.53 (4) &      88.59 (3) &            88.53 (4) & 88.06 (8) &          88.23 (6) & 88.14 (7) &          88.82 (2) & \textbf{88.83 (1)} \\
       361065 & \textbf{86.32 (1)} &      86.09 (4) &            85.79 (6) &  85.6 (7) &          85.55 (8) &  86.3 (2) &          86.04 (5) &          86.19 (3) \\
       361066 &          80.13 (4) &       80.2 (3) &            80.54 (2) & 79.48 (7) &          80.05 (5) & 79.31 (8) &          79.88 (6) & \textbf{80.62 (1)} \\
       361068 &          92.85 (7) &      93.51 (4) &            93.44 (6) & 93.45 (5) &          92.72 (8) & 93.67 (3) & \textbf{93.81 (1)} &          93.72 (2) \\
       361069 &          68.23 (8) &      70.61 (5) &            71.04 (2) & 68.97 (7) &          70.93 (3) & 69.48 (6) &          70.82 (4) & \textbf{71.37 (1)} \\
       361070 &          59.22 (5) &      59.18 (6) &            63.71 (3) & 58.89 (7) &          65.17 (2) & 58.75 (8) &          59.29 (4) & \textbf{65.77 (1)} \\
       361273 & \textbf{60.76 (1)} &      60.57 (4) &            60.53 (6) &  60.5 (7) &          60.49 (8) & 60.54 (5) &          60.59 (3) &          60.67 (2) \\
       361274 &          75.34 (7) &      76.83 (5) &            77.47 (2) & 74.57 (8) &           77.3 (3) & 75.37 (6) &          77.12 (4) & \textbf{78.03 (1)} \\
       361275 &            0.0 (8) &      71.84 (5) &            71.96 (3) & 71.34 (6) &          72.06 (2) & 71.34 (6) &          71.93 (4) & \textbf{72.07 (1)} \\
       361276 &            0.0 (8) &      75.82 (7) &            78.59 (3) &  76.7 (6) & \textbf{79.86 (1)} & 77.06 (4) &          76.87 (5) &          79.31 (2) \\
       361277 &            0.0 (8) &      89.31 (4) &            89.84 (2) & 87.24 (7) &          89.36 (3) & 87.92 (6) &          88.72 (5) & \textbf{90.35 (1)} \\
       361278 & \textbf{73.05 (1)} &      72.67 (2) &            72.35 (6) &  72.4 (4) &           72.1 (8) & 72.41 (3) &          72.37 (5) &          72.16 (7) \\
\midrule
Average Score &              63.71 &           79.0 &                79.85 &     78.02 &              79.84 &     78.37 &              79.03 &              80.13 \\
 Average Rank &               4.94 &           4.12 &                 3.75 &      6.69 &                4.5 &      5.38 &               4.12 &               2.31 \\
\bottomrule
\end{tabular}
}
\end{table*}

\begin{table*}[ht]
\centering
\caption{Additional Datasets: Categorical Regression}
\resizebox{\textwidth}{!}{%
\begin{tabular}{@{}lcccccccc@{}}
\toprule
   Dataset ID &             BiSHop & FT Transformer & GradientBoostingTree &                MLP &       RandomForest &            Resnet &              SAINT &            XGBoost \\
\midrule
       361093 & \textbf{98.98 (1)} &      98.06 (6) &            98.34 (3) &          98.07 (5) &          98.25 (4) &         98.04 (7) &          97.77 (8) &          98.42 (2) \\
       361094 &          99.98 (6) &      99.99 (4) &   \textbf{100.0 (1)} &          99.99 (4) & \textbf{100.0 (1)} &         99.97 (8) &          99.98 (6) & \textbf{100.0 (1)} \\
       361096 &          98.57 (8) &      98.97 (3) &            98.99 (2) &          98.77 (6) &          98.82 (5) &         98.88 (4) &          98.67 (7) & \textbf{99.11 (1)} \\
       361097 &            0.0 (8) &      56.63 (5) &            57.76 (3) &          55.91 (7) &          57.81 (2) &         57.29 (4) &          56.45 (6) & \textbf{57.87 (1)} \\
       361098 &          97.99 (8) &      99.68 (3) &            99.64 (5) &          99.68 (3) &          99.32 (6) &         99.69 (2) &           99.3 (7) &  \textbf{99.8 (1)} \\
       361099 &          94.12 (3) &      94.09 (4) &            94.26 (2) &          93.71 (6) &          93.69 (8) &         93.71 (6) &          93.75 (5) & \textbf{94.77 (1)} \\
       361101 &          49.33 (6) &      52.87 (4) &            58.56 (2) &          47.44 (7) &          58.42 (3) &         49.75 (5) &          46.31 (8) & \textbf{59.13 (1)} \\
       361102 &          83.35 (8) &      89.34 (2) &            89.28 (3) &          87.57 (6) &          87.53 (7) &         88.52 (4) &          88.36 (5) & \textbf{89.77 (1)} \\
       361103 &           63.2 (8) &      67.02 (4) &            68.57 (2) &          65.99 (7) &          67.47 (3) &         66.12 (5) &          66.02 (6) & \textbf{69.14 (1)} \\
       361104 &          99.94 (7) &      99.97 (5) &   \textbf{99.98 (1)} & \textbf{99.98 (1)} & \textbf{99.98 (1)} &         99.96 (6) &           99.9 (8) & \textbf{99.98 (1)} \\
       361287 &          -2.82 (8) &       5.33 (5) &             5.34 (4) &           4.15 (7) &  \textbf{7.36 (1)} &          5.06 (6) &           6.05 (3) &           6.94 (2) \\
       361288 &          57.96 (3) &      57.48 (4) &            55.75 (7) &          58.03 (2) &          55.79 (6) & \textbf{58.3 (1)} &          57.09 (5) &          55.75 (7) \\
       361289 &          10.91 (8) &      18.01 (6) &   \textbf{18.65 (1)} &          17.23 (7) &          18.28 (3) &         18.05 (5) &          18.22 (4) &          18.55 (2) \\
       361291 &           1.45 (8) &       6.88 (4) &              7.5 (3) &           6.26 (6) &           7.67 (2) &          6.09 (7) &           6.72 (5) &  \textbf{7.84 (1)} \\
       361292 &          50.96 (7) &      52.01 (4) &            53.04 (2) &          51.58 (5) &           49.7 (8) &         51.41 (6) &           52.6 (3) & \textbf{53.65 (1)} \\
       361293 &          -8.96 (8) &       4.67 (3) &    \textbf{4.86 (1)} &           4.17 (7) &           4.58 (4) &           4.2 (6) &           4.54 (5) &           4.85 (2) \\
       361294 &          96.76 (8) &      97.93 (3) &            97.94 (2) &          97.92 (5) &          97.88 (7) &         97.93 (3) & \textbf{97.96 (1)} &          97.89 (6) \\
\midrule
Average Score &              58.34 &          64.64 &                 65.2 &              63.91 &              64.86 &             64.29 &               64.1 &               65.5 \\
 Average Rank &               6.65 &           4.06 &                 2.59 &               5.35 &               4.18 &               5.0 &               5.41 &               1.88 \\
\bottomrule
\end{tabular}
}
\end{table*}

\begin{table*}[ht]
\centering
\caption{Additional Datasets: Numerical Regression}
\resizebox{\textwidth}{!}{%
\begin{tabular}{@{}lcccccccc@{}}
\toprule
   Dataset ID &             BiSHop &     FT Transformer & GradientBoostingTree &                MLP &      RandomForest &    Resnet &              SAINT &            XGBoost \\
\midrule
       361072 &           96.9 (8) &          98.48 (4) &            98.61 (2) &          97.91 (7) &         98.26 (5) & 98.26 (5) &          98.51 (3) & \textbf{98.62 (1)} \\
       361073 &          99.49 (3) & \textbf{99.51 (1)} &             99.0 (5) &          97.31 (7) &         98.67 (6) & 96.19 (8) & \textbf{99.51 (1)} &          99.15 (4) \\
       361074 &          87.65 (6) &          91.83 (2) &            85.07 (7) &          91.81 (3) &          83.3 (8) & 91.56 (4) & \textbf{91.86 (1)} &          90.76 (5) \\
       361076 &          36.62 (7) &          37.15 (6) &            47.74 (3) &          39.61 (4) &         48.07 (2) & 38.21 (5) &          36.32 (8) & \textbf{50.06 (1)} \\
       361077 &           82.4 (5) &          73.28 (6) &   \textbf{83.97 (1)} &          83.72 (2) &         83.72 (2) & 71.85 (7) &           70.1 (8) &          83.66 (4) \\
       361078 &          76.91 (8) &          83.52 (3) &            83.95 (2) &          80.97 (7) &          82.7 (5) &  83.1 (4) &          81.39 (6) & \textbf{85.22 (1)} \\
       361079 & \textbf{60.76 (1)} &          53.09 (4) &            57.45 (2) &          48.62 (7) &         50.16 (6) & 51.77 (5) &          46.79 (8) &          55.42 (3) \\
       361080 &          93.45 (8) &          94.36 (5) &            94.52 (2) &          94.41 (4) &         93.94 (7) & 94.45 (3) &          94.22 (6) & \textbf{94.56 (1)} \\
       361081 &          98.67 (8) &          99.69 (2) &            99.65 (4) &          99.52 (5) &         99.31 (7) & 99.67 (3) &          99.38 (6) & \textbf{99.76 (1)} \\
       361082 &          65.32 (8) &           68.1 (4) &            69.23 (2) &          67.71 (5) &          67.2 (6) & 67.18 (7) &          68.16 (3) & \textbf{69.61 (1)} \\
       361083 &          48.65 (5) &          49.87 (4) &            55.27 (2) &          46.79 (8) &          54.6 (3) &  48.2 (6) &          47.13 (7) & \textbf{55.37 (1)} \\
       361084 &          80.45 (8) &           88.1 (2) &             88.0 (3) &          85.72 (7) &         86.89 (5) &  86.8 (6) &          87.31 (4) & \textbf{88.92 (1)} \\
       361085 &          81.71 (6) &          81.01 (7) &             82.1 (5) &          86.83 (2) &         84.39 (4) & 85.43 (3) &          78.59 (8) & \textbf{86.87 (1)} \\
       361086 &          95.14 (8) &          97.93 (2) &   \textbf{97.94 (1)} &          97.91 (4) &         97.68 (7) & 97.93 (2) &          97.88 (5) &          97.88 (5) \\
       361087 &          84.79 (8) &          92.59 (2) &            92.57 (3) &          90.91 (7) &         91.41 (6) &  91.7 (4) &          91.58 (5) & \textbf{93.66 (1)} \\
       361088 &          87.98 (8) &          89.03 (7) &            90.32 (2) &          89.65 (4) &         90.11 (3) & 89.53 (5) &          89.09 (6) & \textbf{91.06 (1)} \\
       361279 &           0.59 (8) &           5.35 (5) &             5.57 (4) &           2.23 (7) & \textbf{9.39 (1)} &  4.28 (6) &           5.95 (3) &           8.29 (2) \\
       361280 &           56.9 (4) &          57.48 (3) &            54.87 (8) & \textbf{58.46 (1)} &         55.27 (7) & 57.81 (2) &          56.84 (5) &          55.49 (6) \\
       361281 &          -1.26 (8) &           2.11 (5) &             2.77 (3) &           1.51 (6) & \textbf{3.15 (1)} &  1.29 (7) &           2.21 (4) &           3.04 (2) \\
\midrule
Average Score &              70.16 &              71.71 &                73.08 &              71.66 &             72.54 &     71.33 &              70.67 &              74.07 \\
 Average Rank &               6.58 &               3.89 &                 3.21 &               5.11 &              4.79 &      4.84 &               5.11 &               2.21 \\
\bottomrule
\end{tabular}
}
\end{table*}
